# Supplementary material for: Improving Minimum Bayes Risk Decoding with Multi-Prompt
Source: arXiv:2407.15343 source file (2024-10-03)
Supplement: Supplementary file 1 [file prompt_distribution.tex]

\begin{figure}[t!]
\centering
\includegraphics[width=0.47\textwidth]{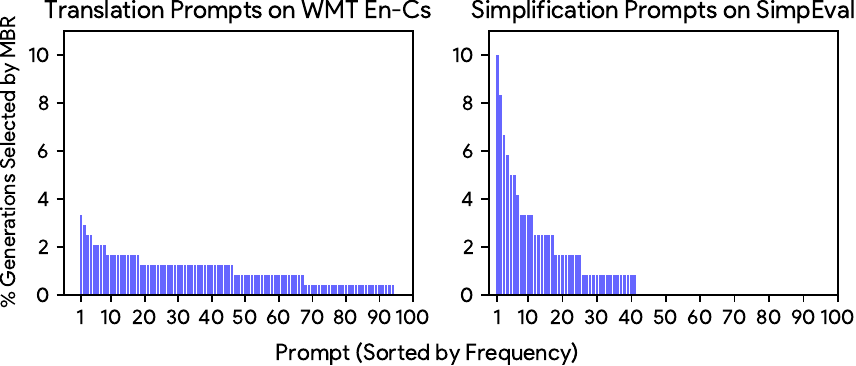}
\setlength{\abovecaptionskip}{8pt}
\setlength{\belowcaptionskip}{-10pt}
\captionof{figure}{Distribution of prompt usage for 100 prompts. A few high quality prompts generate many final candidates, while many prompts are rarely (if ever) used.}
\label{fig:prompt_distribution}
\end{figure}
