# Supplementary material for: Improving Minimum Bayes Risk Decoding with Multi-Prompt
Source: arXiv:2407.15343 source file (2024-10-03)
Supplement: Supplementary file 2 [file candidate_similarity.tex]

\setlength{\tabcolsep}{2pt}
\begin{table}[t!]
\centering
\fontsize{8}{9.5}\selectfont

\begin{tabular}{p{60pt}C{45pt}C{45pt}C{45pt}}

\toprule
% \textbf{Method} & \textbf{Improvement (MP over SP)} & \textbf{\textsc{Bleu} (MP on SP)} & \textbf{\textsc{Bleu} (SP on MP)} \\
& Metric Improvement & Cand. \textsc{Bleu} (MP on SP) & Cand. \textsc{Bleu} (SP on MP) \\
\midrule
\multicolumn{4}{l}{\textit{Code Generation} ($|\mathcal{H}|\!=\!20$) -- \textsc{HumanEval} (pass@1)} \\
\hdashrule
StarCoder 2 15B & \plus{4.88} & 49.69 & 50.13 \\
CodeLlama 7B    & \plus{3.05} & 62.05 & 63.32 \\
CodeLlama 13B   & \plus{4.88} & 59.49 & 60.76 \\
CodeLlama 34B   & \plus{6.71} & 61.59 & 62.92 \\
CodeLlama 70B   & \plus{7.31} & 63.15 & 65.12 \\
GPT-3.5         & \plus{5.49} & 83.07 & 89.86 \\
GPT-4           & \plus{1.22} & 81.72 & 89.82 \\
\midrule
\multicolumn{4}{l}{\textit{Text Simplification} ($|\mathcal{H}|\!=\!100$) -- \textsc{SimpEval} (LENS)} \\
\hdashrule
Llama 2 7B Chat     & \plus{4.67} & 80.71 & 74.68 \\
Llama 2 13B Chat    & \plus{2.08} & 79.30 & 77.65 \\
Llama 2 70B Chat    & \plus{1.07} & 74.11 & 70.65 \\
GPT-3.5             & \plus{4.38} & 94.18 & 85.56 \\
GPT-4               & \plus{5.09} & 96.74 & 81.05 \\
\midrule
\multicolumn{4}{l}{\textit{Translation} ($|\mathcal{H}|\!=\!100$) -- WMT '22 \textsc{En-Cs} (COMET)} \\
\hdashrule
ALMA 7B R   & \plus{0.77} & 87.22 & 81.20 \\
ALMA 13B R  & \plus{1.04} & 89.75 & 84.74 \\
GPT-3.5     & \plus{0.08} & 99.26 & 95.47 \\
GPT-4       & \plus{0.23} & 90.21 & 90.85 \\

\bottomrule
\end{tabular}
\setlength{\belowcaptionskip}{-10pt}
\caption{Candidate set overlap for state-of-the-art models tested in Table \ref{table:multi_model}. `Candidate \textsc{Bleu}' measures the \textsc{Bleu} score for multi-prompt candidates using single-prompt as references and vice-versa.}
\label{table:candidate_similarity}
\end{table}
